# Supplementary material for: Kempe Swap K-Means: A Scalable Near-Optimal Solution for Semi-Supervised Clustering
Source: arXiv:2603.27417 source file (2026-03-28)
Supplement: Supplementary file 1 [file First_Descent.tex]

\subsubsection{Kempe Swap Assignment First Descent Variants}

\begin{center}
\resizebox{0.7\linewidth}{!}{%
\begin{algorithm}[H]
\caption{Local Search with Kempe Chain Neighborhood: $LS(V, E,L, U)$}
\label{alg:LSKC}
\DontPrintSemicolon
\SetKwInOut{Input}{Input}\SetKwInOut{Output}{Output}
\Input{
Graph $G=(V,E)$, data $\{(y_i,w_i),v_i \in V\}$;\\
Number of iterations $L$;\\
Initial cluster assignments $U = \{u(v_i)\}_{i=1}^{n}$.
}
\Output{New Cluster assignments $\{u(v_i)\}_{i=1}^{n}$}
\BlankLine
Reorganizing data into cluster matrices $\{W_k = [w_i: u(v_i)=k]\}_{k=1}^K$,  $\{Y_k = [y_i: u(v_i)=k]\}_{k=1}^K$\;
Initialize centroids  $\{\beta_k = f(W_k,Y_k)\}_{k=1}^K$\;
Compute sum of residual per cluster $\{J_k=\sum_{i:u(v_i = k)} \|y_i - w_i\beta_k\|^2\}_{k=1}^K$\;
Tabu list $\tau = \emptyset$\;

\BlankLine

\For{$1$ to $L$}{
$flag = 0$\;
Sort the cluster by sum of residual per cluster in decreasing order $\{C_{key_k}\}_{k=1}^K$\;
\tcp{Neighborhood search}
\For{$i \in \{key_1,key_2,\cdots,key_K\}$}{
\If{$flag$}{Break loop\;}
\For{$j \in \{key_{i+1},key_{i+2},\cdots,key_K\}$}{
\If{$(i,j) \notin \tau$ and $(j,i) \notin \tau$}{
Partition $C_i \cup C_j \cap G$ into maximal connected subgraphs $\mathbb{H} = \{H_1, H_2,\cdots\}$\;
\tcp{$K$-Means optimization between two clusters}
\While{not converged}{
\For{$H \in \mathbb{H}$}{
Split vertices $H^i = H\cap C_i, \quad H^j = H\cap C_j$\;
\If{$\sum_{p\in H^i}(\|y_p - w_p\beta_j\|^2 - \|y_p - w_p\beta_i\|^2) + \sum_{q\in H^j}(\|y_q - w_q\beta_i\|^2 - \|y_q - w_q\beta_j\|^2) < 0$}{
Update cluster assignments $C_i = C_i\cup H^j\setminus H^i, \quad C_j = C_j\cup H^i\setminus H^j$\;
$flag = 1$\;
}
}
Update centroids $\beta_i,\beta_j$\;
}

\eIf{$flag$}{
Update Tabu list $\tau = \tau\setminus\{(p,q), \forall i,j \in (p,q)\} +\{(i,j)\}$\; 
Re-label the cluster by sum of residual per cluster in decreasing order $\{C_{k}\}_{k=1}^K$\;
Break loop\;
}
{Update Tabu list $\tau = \tau +\{(i,j)\}$\; }
}
}
}
\If{not $flag$}{\tcp{Local optimal}Break loop\;}
}
\Return Cluster assignments $\{u(v_i)\}_{i=1}^{n}$
\end{algorithm}
}
\end{center}
