# Supplementary material for: Kempe Swap K-Means: A Scalable Near-Optimal Solution for Semi-Supervised Clustering
Source: arXiv:2603.27417 source file (2026-03-28)
Supplement: Supplementary file 2 [file SDP_Initialization.tex]

\subsection{SDP Initialization}
\cite{piccialli2022sos} extends the semidefinite programming formulation on clustering proposed by \cite{peng2007approximating} to constrained clustering and shows the equivalence between formulation (\ref{eq:1}) and (\ref{eq:2}).
\begin{subequations}\label{eq:2}
\begin{align}
    \min_{Z} \quad & \mathrm{tr}\big(W(I - Z)\big) \tag{\ref{eq:2}}\\
    \text{s.t.} \quad 
    & Ze = e,\ \mathrm{tr}(Z) = k, \label{eq:2a}\\
    & Z_{ih} = Z_{jh}, \quad && \forall h \in [n],\ \forall (i,j) \in \mathcal{ML}, \label{eq:2b}\\
    & Z_{ij} = 0, \quad && \forall (i,j) \in \mathcal{CL}, \label{eq:2c}\\
    & Z \ge 0,\ Z^2 = Z,\ Z = Z^\top,\label{eq:2d}
\end{align}
\end{subequations}
where decision matrix $Z = X(XX^\top)^{-1}X^\top$ and affinity $W_{i,j} = y_i^{\top}y_j$. 

% Randomization helps addressing the first problem of local optima. Kempe Chain Swap $K$-Means can starts with different initial clustering, whether Kempe-equivalent or not or randomly exclude improving swaps in finding another local optima. 
Algorithm \ref{alg:KCSKM} ($KSKM$) initializes the cluster assignments in lines 1–3. It begins by obtaining a feasible clustering using the DSATUR algorithm \citep{brelaz1979new}. The DSATUR algorithm greedily colors vertices based on their degree of saturation, which measures how constrained a vertex is given the current partial coloring. As DSATUR generally produces a number of colors close to the chromatic number, we expand the clustering to a $k$-coloring by repeatedly bisecting the cluster with the highest SSE.
To obtain an effective set of initial cluster centroids, we follow the approach of \cite{piccialli2022sos}, which approximates the solution of a relaxed version of the SDP problem (\ref{eq:2}) using a $k$-rank matrix:

\begin{subequations}\label{eq:6} 
\begin{align} \min_{Z} \quad & \mathrm{tr}\big(W(I - Z)\big) \tag{\ref{eq:6}}\\ 
\text{s.t.} \quad & Ze = e,\ \mathrm{tr}(Z) = k, \label{eq:6a}\\ 
& Z_{ih} = Z_{jh}, \quad && \forall h \in [n],\ \forall (i,j) \in \mathcal{ML}, \label{eq:6b}\\ 
& Z_{ij} = 0, \quad && \forall (i,j) \in \mathcal{CL}, \label{eq:6c}\\ & 
Z \ge 0,\ Z\succ 0.\label{eq:6d} 
\end{align} 
\end{subequations}

They show that the constraints (\ref{eq:2d}) can be replaced by $Z \ge 0$, $Z \succ 0$, and $\mathrm{rank}(Z) = k$.
Let $Z_{\text{SDP}}$ denote the solution to the relaxed problem (\ref{eq:6}), and let $\hat{Z}$ be its best rank-$k$ approximation. The approximate cluster centroids can then be obtained by applying unconstrained $K$-Means to the transformed data $\hat{Z}W$.
If the relaxation (\ref{eq:6}) is tight, the unique rows of $\hat{Z}W$ coincide exactly with the centroids of the optimal clustering.

The best rank-$k$ approximation $\hat{Z}$ is computed as follows:
\begin{equation*}
\min_{\hat{Z}} \quad ||\hat{Z} - Z_{\text{SDP}}||_{F}
\quad \text{s.t.} \quad \mathrm{rank}(\hat{Z}) = k,
\end{equation*}
whose solution is given by the truncated singular value decomposition (SVD) of $Z{\text{SDP}}$.

Both \cite{piccialli2022exact} and \cite{piccialli2022sos} demonstrated that SDP-based centroid initialization leads to favorable local optima for centroid-based iterative algorithms such as COP-$K$-Means \citep{wagstaff2001constrained} and $BLPKM_{CC}$ \citep{baumann2020}.
However, because solving the SDP relaxation is computationally expensive, we include the SDP-based centroid initialization in $KSKM$ as an optional component. Since $KSKM$ can achieve robust performance through a top-down process that repeatedly splits clusters until the desired number of clusters $k$ is reached, we recommend using the SDP-based initialization only when the number of clusters identified by DSATUR is close to $k$. Alternatively, the SDP-based initialization can be replaced with a simpler, unconstrained clustering-based initialization.
Once the target centroids are determined, the initial cluster assignments are shifted toward the target centroids using Algorithm \ref{alg:KSShift} $KSShift$.
